# Supplementary material for: Fast Approximate Geodesics for Deep Generative Models
Source: arXiv:1812.08284 source file (2019-05-23)
Supplement: Supplementary file 1 [file appendix.tex]

\newpage
\cleardoublepage
\onecolumn
